# Supplementary material for: Pre-Trained Language Models for Interactive Decision-Making
Source: arXiv:2202.01771 source file (2022-10-29)
Supplement: Supplementary file 1 [file goal_predictes_list.tex]

\begin{figure*}[h]
\centering
\hfill
\begin{minipage}{0.48\textwidth}
    \captionof{table}{\small{ \textbf{Goal predicates used in the \emph{In-Distribution} and \emph{Novel Scenes} settings.}}}
    % \vspace{-10pt}
    \label{tbl:normal_predicates}
    \begin{center}
    \small
    \setlength{\tabcolsep}{3pt}
    % \resizebox{1\textwidth}{!}{
    \begin{tabular}{l}
    \toprule
    \texttt{ON(cutleryfork, kitchentable):$0\sim3$} \\
    \texttt{ON(plate, kitchentable):$0\sim3$} \\
    \texttt{ON(waterglass, kitchentable):$0\sim3$} \\
    \texttt{ON(wineglass, kitchentable):$0\sim3$} \\
    
    \texttt{INSIDE(cutleryfork, dishwasher):$0\sim3$} \\
    \texttt{INSIDE(plate, dishwasher):$0\sim3$} \\
    \texttt{INSIDE(waterglass, dishwasher):$0\sim3$} \\
    \texttt{INSIDE(wineglass, dishwasher):$0\sim3$} \\
    
    \texttt{INSIDE(cutleryfork, sink):$0\sim3$} \\
    \texttt{INSIDE(plate, sink):$0\sim3$} \\
    \texttt{INSIDE(waterglass, sink):$0\sim3$} \\
    \texttt{INSIDE(wineglass, sink):$0\sim3$} \\
    
    \texttt{INSIDE(milk, fridge):$0\sim3$} \\
    \texttt{INSIDE(chicken, fridge):$0\sim3$} \\
    \texttt{INSIDE(cupcake, fridge):$0\sim3$} \\
    \texttt{INSIDE(pancake, fridge):$0\sim3$} \\
    \texttt{INSIDE(poundcake, fridge):$0\sim3$} \\
    
    \texttt{ON(milk, kitchentable):$0\sim3$} \\
    \texttt{ON(chicken, kitchentable):$0\sim3$} \\
    \texttt{ON(cupcake, kitchentable):$0\sim3$} \\
    \texttt{ON(pancake, kitchentable):$0\sim3$} \\
    \texttt{ON(poundcake, kitchentable):$0\sim3$} \\
    
    \texttt{INSIDE(chicken, microwave):$0\sim3$} \\
    \texttt{INSIDE(cupcake, microwave):$0\sim3$} \\
    \texttt{INSIDE(pancake, microwave):$0\sim3$} \\
    \texttt{INSIDE(poundcake, microwave):$0\sim3$} \\
    
    \texttt{INSIDE(chicken, oven):$0\sim3$} \\
    \texttt{INSIDE(cupcake, oven):$0\sim3$} \\
    \texttt{INSIDE(pancake, oven):$0\sim3$} \\
    \texttt{INSIDE(poundcake, oven):$0\sim3$} \\
    
    \texttt{CLOSE(oven):$0\sim1$} \\
    \texttt{CLOSE(dishwasher):$0\sim1$} \\
    \texttt{CLOSE(microwave):$0\sim1$} \\
    \texttt{CLOSE(fridge):$0\sim1$} \\
    
    \texttt{TurnON(oven):$0\sim1$} \\
    \texttt{TurnON(dishwasher):$0\sim1$} \\
    \texttt{TurnON(microwave):$0\sim1$} \\
    
    % 37
    \bottomrule
    \end{tabular}
    % }
    \end{center}
    \end{minipage}%
    \hfill
    \begin{minipage}{0.48\textwidth}
    \captionof{table}{\small{\textbf{Goal predicates used in the \emph{Novel Tasks} setting.}}}
    % \vspace{-10pt}
    \label{tbl:zero_shot_predicates}
    \begin{center}
    \small
    \setlength{\tabcolsep}{3pt}
    % \resizebox{1\textwidth}{!}{
    \begin{tabular}{l}
    \toprule
    \texttt{INSIDE(milk, dishwasher):$0\sim3$} \\
    \texttt{INSIDE(chicken, dishwasher):$0\sim3$} \\
    \texttt{INSIDE(cupcake, dishwasher):$0\sim3$} \\
    \texttt{INSIDE(pancake, dishwasher):$0\sim3$} \\
    
    \texttt{ON(milk, sink):$0\sim3$} \\
    \texttt{ON(chicken, sink):$0\sim3$} \\
    \texttt{ON(cupcake, sink):$0\sim3$} \\
    \texttt{ON(pancake, sink):$0\sim3$} \\
    
    \texttt{INSIDE(cutleryfork, fridge):$0\sim3$} \\
    \texttt{INSIDE(plate, fridge):$0\sim3$} \\
    \texttt{INSIDE(waterglass, fridge):$0\sim3$} \\
    \texttt{INSIDE(wineglass, fridge):$0\sim3$} \\
    
    \texttt{INSIDE(cutleryfork, microwave):$0\sim3$} \\
    \texttt{INSIDE(plate, microwave):$0\sim3$} \\
    \texttt{INSIDE(waterglass, microwave):$0\sim3$} \\
    \texttt{INSIDE(wineglass, microwave):$0\sim3$} \\
    \texttt{INSIDE(milk, microwave):$0\sim3$} \\
    
    \texttt{INSIDE(cutleryfork, oven):$0\sim3$} \\
    \texttt{INSIDE(plate, oven):$0\sim3$} \\
    \texttt{INSIDE(waterglass, oven):$0\sim3$} \\
    \texttt{INSIDE(wineglass, oven):$0\sim3$} \\
    \texttt{INSIDE(milk, oven):$0\sim3$} \\
    % 22
    \bottomrule
    \end{tabular}
    % }
    \end{center}
    \end{minipage}
\vspace{-15pt}
\end{figure*}
