# Supplementary material for: Pre-Trained Language Models for Interactive Decision-Making
Source: arXiv:2202.01771 source file (2022-10-29)
Supplement: Supplementary file 2 [file baseline-lstm.tex]

\begin{figure}[h]
\begin{center}
\includegraphics[width=\linewidth]{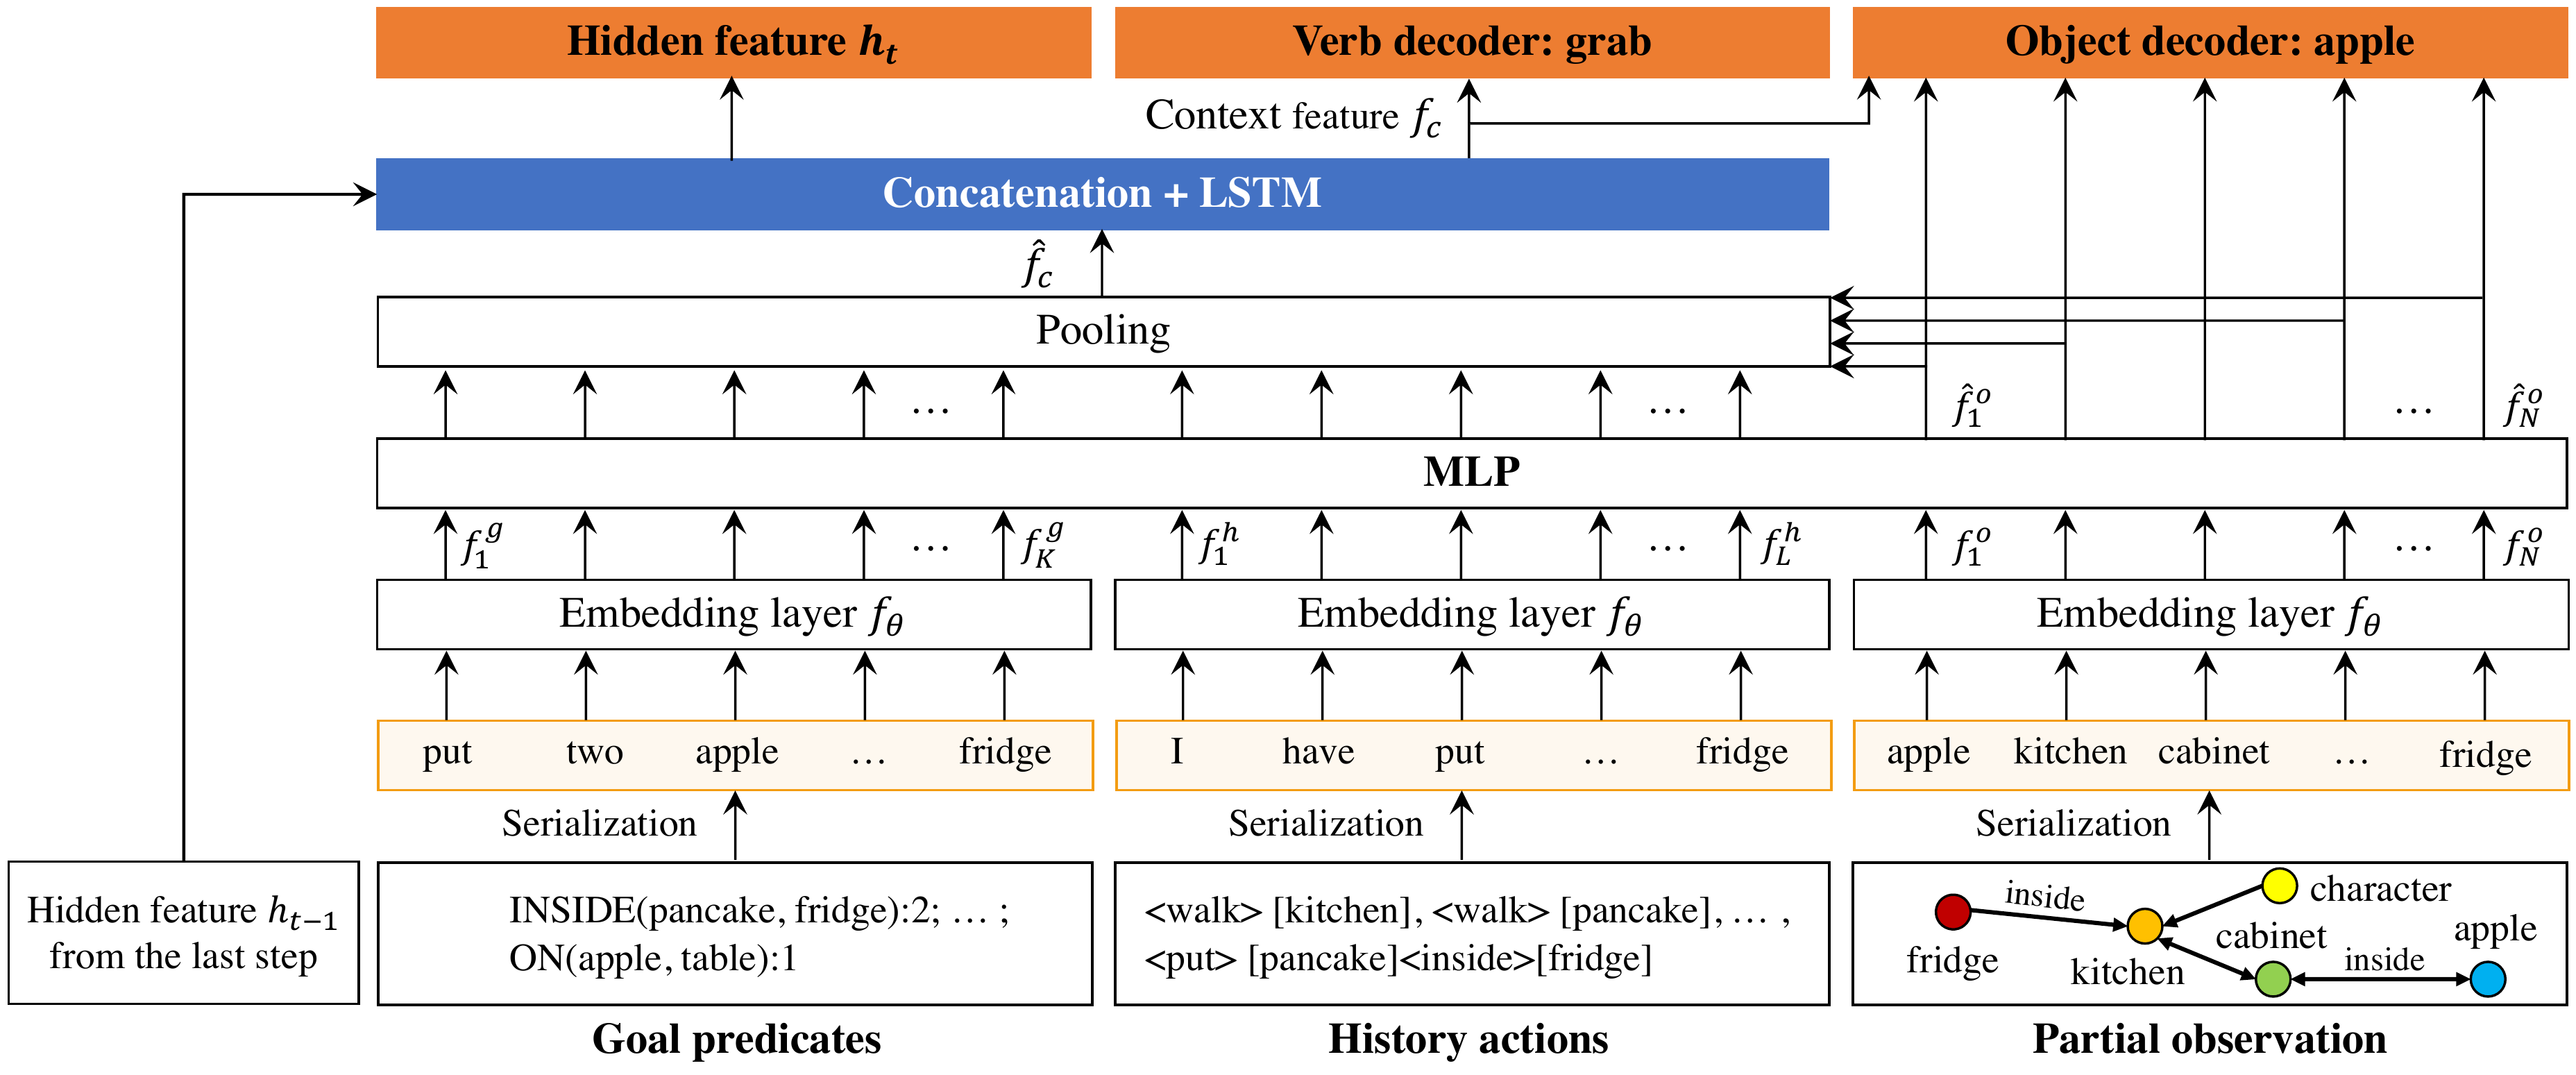}
\end{center}
\vspace{-10pt}
\caption{\small \textbf{Baseline LSTM.}
The input and output are the same as ``LM (ft)'' as we introduced in the main paper \sect{exp:exp1} and this appendix \sect{apx:model_architecture}.
``LSTM'' has a similar architecture as ``MLP-N'' in \fig{apx_fig:mlp-n}.
The difference is in the ways to compute the context feature $f_c$.
The feature $\hat{f}_c$ after the pooling layer is first concatenated with the hidden feature $h_{t-1}$ from the last step and then sent to LSTM \citep{hochreiter1997long}.
LSTM outputs the context feature $f_c$ and a hidden feature $h_t$ that will be used for the next step.
The verb decoder and object decode are the same as ``MLP-N''.
}
\label{apx_fig:lstm}
\vspace{-10pt}
\end{figure}
