# Supplementary material for: Pre-Trained Language Models for Interactive Decision-Making
Source: arXiv:2202.01771 source file (2022-10-29)
Supplement: Supplementary file 3 [file baseline-mlp-1.tex]

\begin{figure}[h]
\begin{center}
\includegraphics[width=\linewidth]{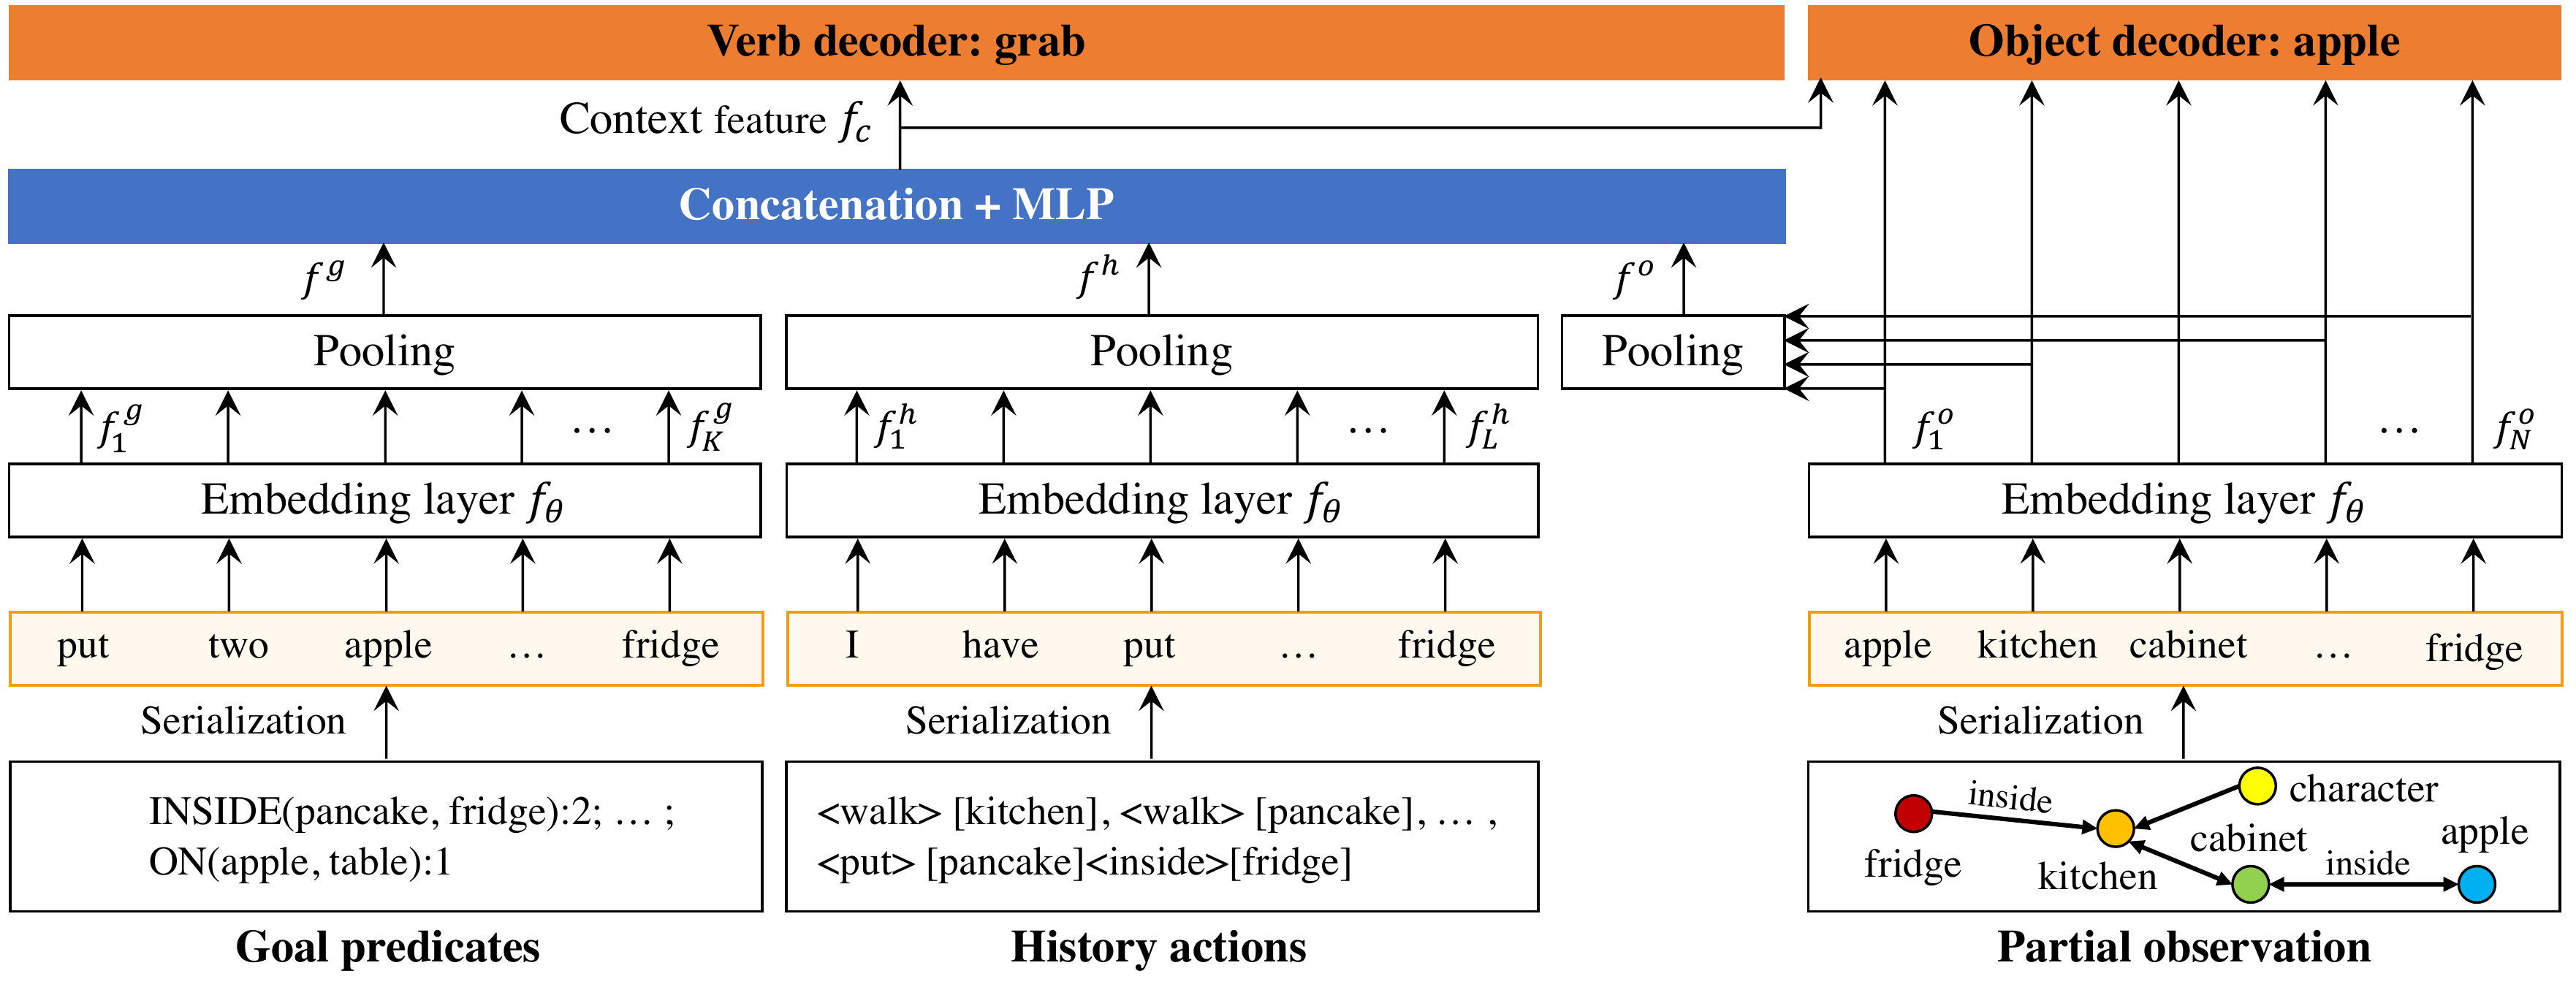}
\end{center}
\vspace{-10pt}
\caption{\small \textbf{Baseline MLP-1.}
The input and output are the same as ``LM (ft)'' as we introduced in the main paper \sect{exp:exp1} and this appendix \sect{apx:model_architecture}.
``MLP-1'' obtains an averaged feature $f_g$ of the task goal by averaging the features of all the tokens in the goal sentences $\{f^g_1, \cdots, f^g_K\}$.
Similarly, ``MLP-1'' obtains an averaged feature of the history $f_h$ and an averaged feature of the observation $f_o$ by averaging the features of all the tokens in the history sentences $\{f^h_1, \cdots, f^h_L\}$ and all the observed objects $\{f^o_1, \cdots, f^o_N\}$, respectively. 
The averaged goal feature $f_g$, the averaged history feature $f_h$, and the averaged observation feature $f_o$ are concatenated and sent to an MLP to generate the context feature $f_c$. 
The MLP consists of two fully-connected layers with a ReLU layer in the middle.
The verb decoder takes the context feature $f_c$ as input and outputs a verb prediction. Different from ``LM (ft)'', the object decoder takes the object features right after the ``Embedding layer $f_{\theta}$'' box as input to predicate the interacted object.
}
\label{apx_fig:mlp-1}
\vspace{-10pt}
\end{figure}
