# Supplementary material for: Pre-Trained Language Models for Interactive Decision-Making
Source: arXiv:2202.01771 source file (2022-10-29)
Supplement: Supplementary file 4 [file baseline-mlp-n.tex]

\begin{figure}[h]
\begin{center}
\includegraphics[width=0.7\linewidth]{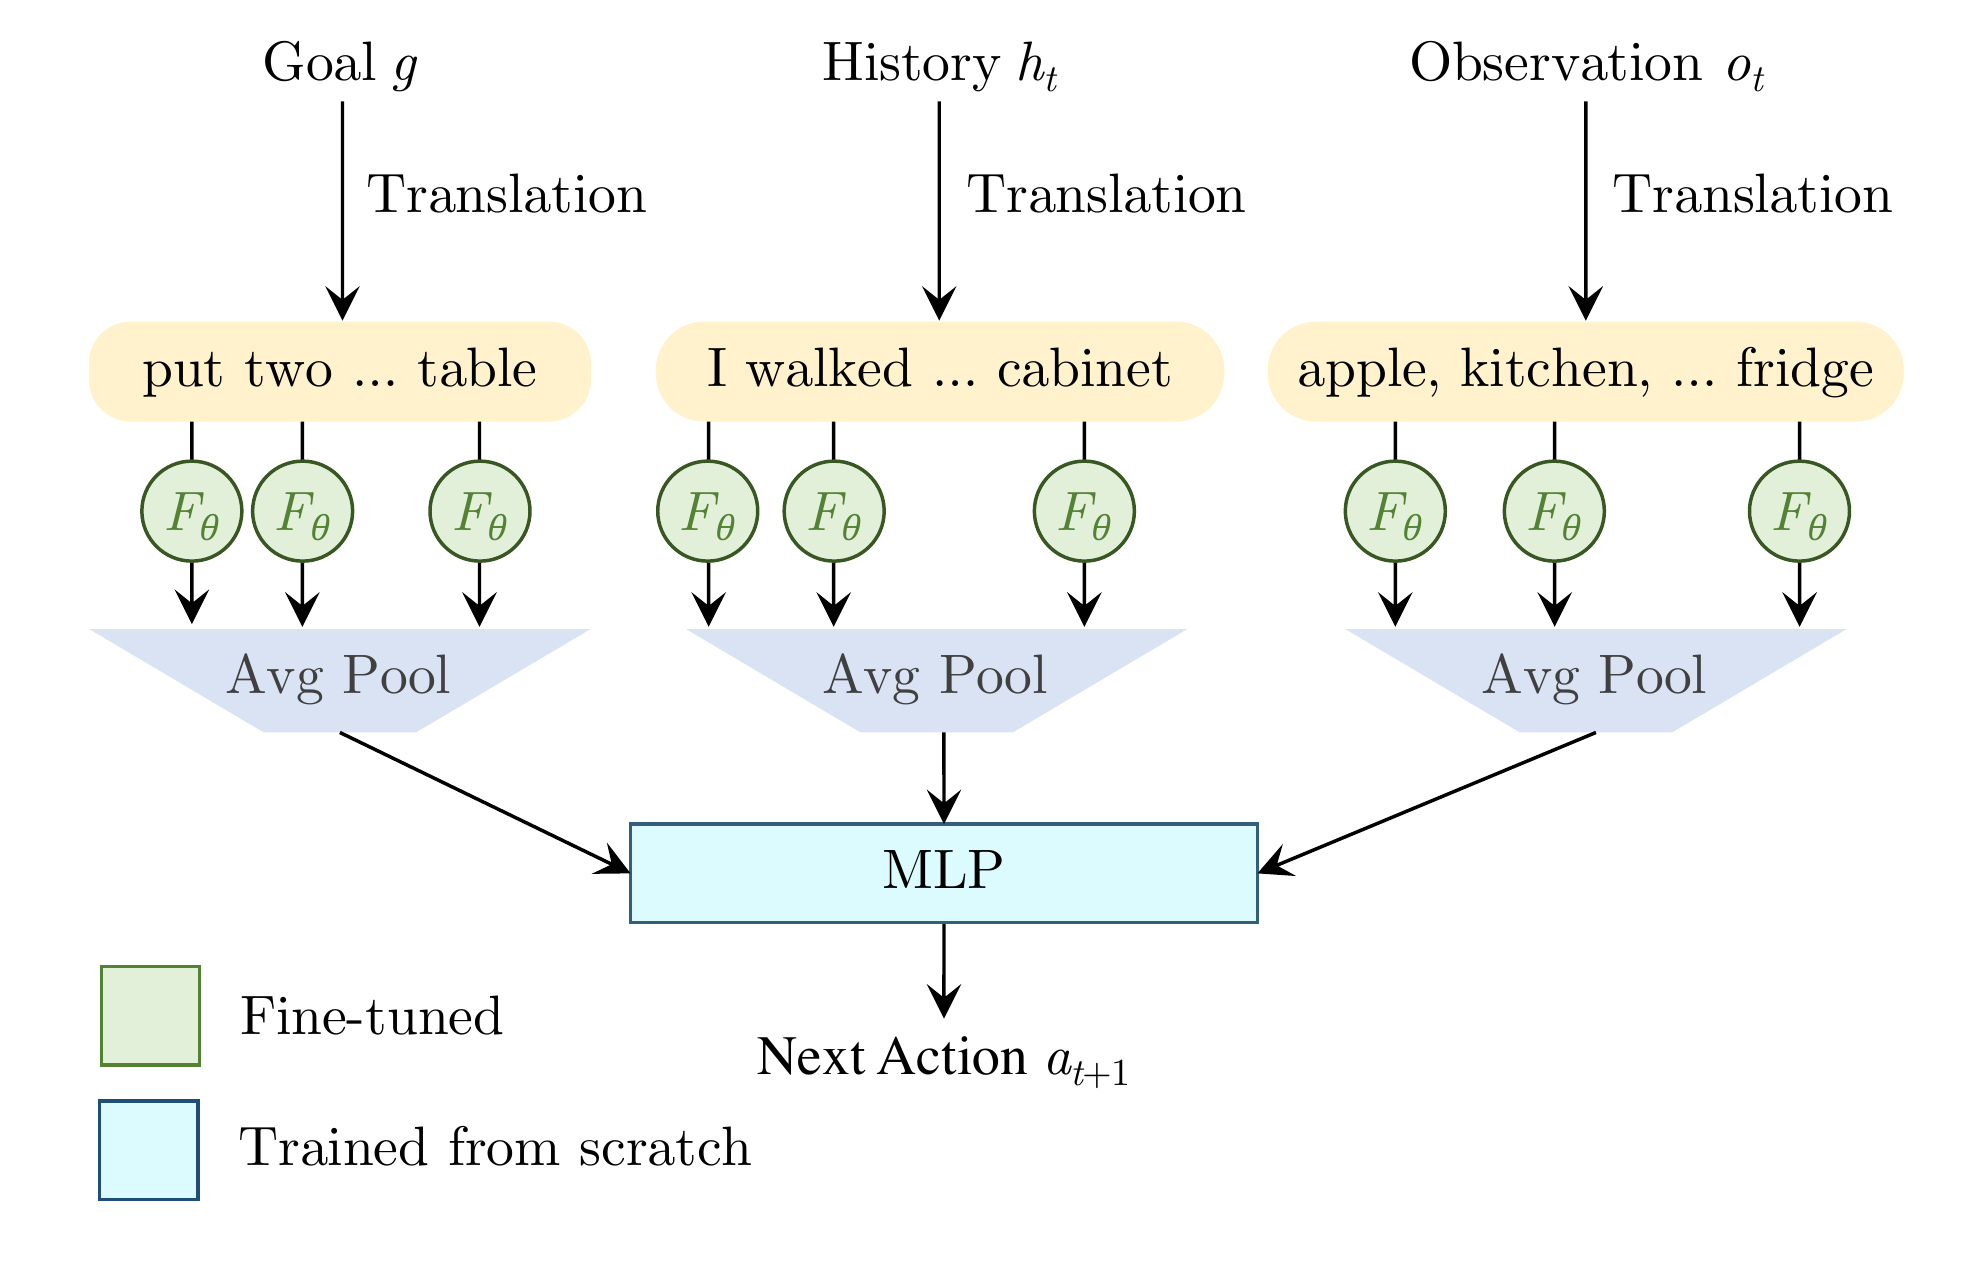}
\end{center}
\vspace{-10pt}
\caption{\small \textbf{Baseline MLP-N.} 
The input and output are the same as ``LM (ft)'' as we introduced in the main paper \sect{exp:exp1} and this appendix \sect{apx:model_architecture}.
The difference is that instead of sending the concatenated features of the goal, history, and observation to the pre-trained language model, ``MLP-N'' sends them to an MLP followed by an average pooling layer to generate the context feature $f_c$.
The MLP consists of two fully-connected layers with a ReLU layer in the middle.
The verb decoder and object decode are the same as ``LM (ft)''.}
\label{apx_fig:mlp-n}
\vspace{-10pt}
\end{figure}
