# Supplementary material for: Pre-Trained Language Models for Interactive Decision-Making
Source: arXiv:2202.01771 source file (2022-10-29)
Supplement: Supplementary file 6 [file repgoal.tex]

\begin{figure}
\begin{center}
\includegraphics[width=1\linewidth]{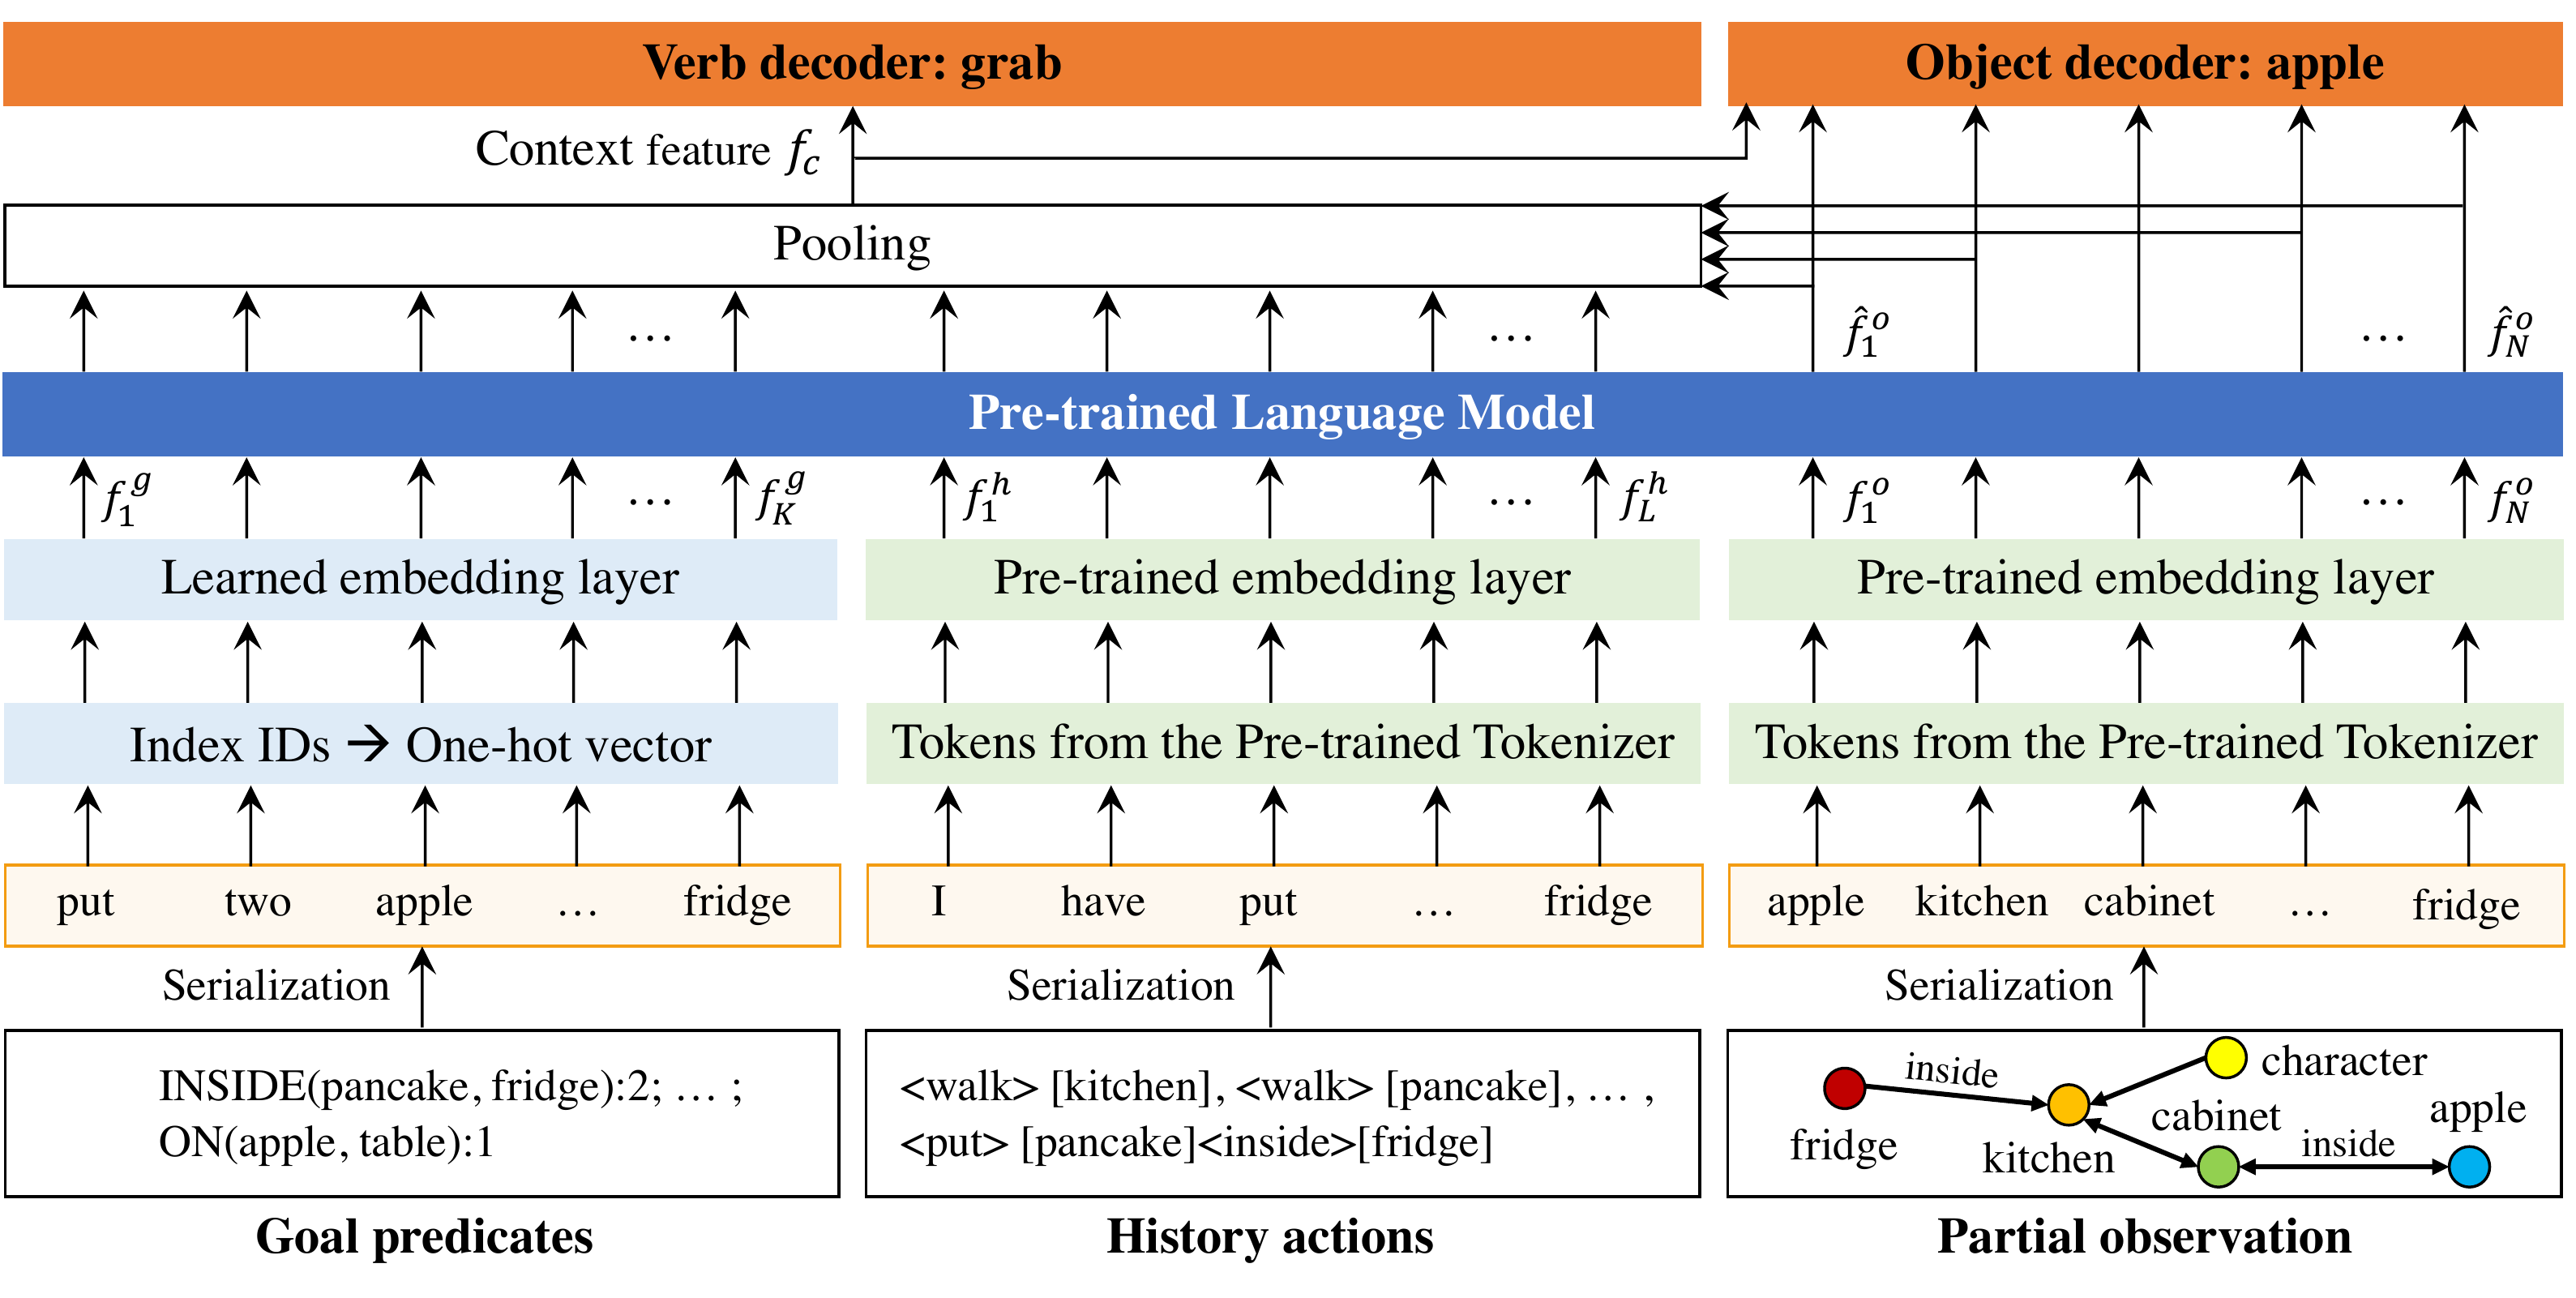}
\end{center}
\vspace{-12pt}
\caption{\small \textbf{Model architecture of ``rep Goal'' used in the main paper \sect{sect:pre-trained-learned-encoding}}.}
\label{fig:model_repgoal}
\vspace{-10pt}
\end{figure}
