# Supplementary material for: Pre-Trained Language Models for Interactive Decision-Making
Source: arXiv:2202.01771 source file (2022-10-29)
Supplement: Supplementary file 8 [file repno.tex]

\begin{figure}
\begin{center}
\includegraphics[width=0.7\linewidth]{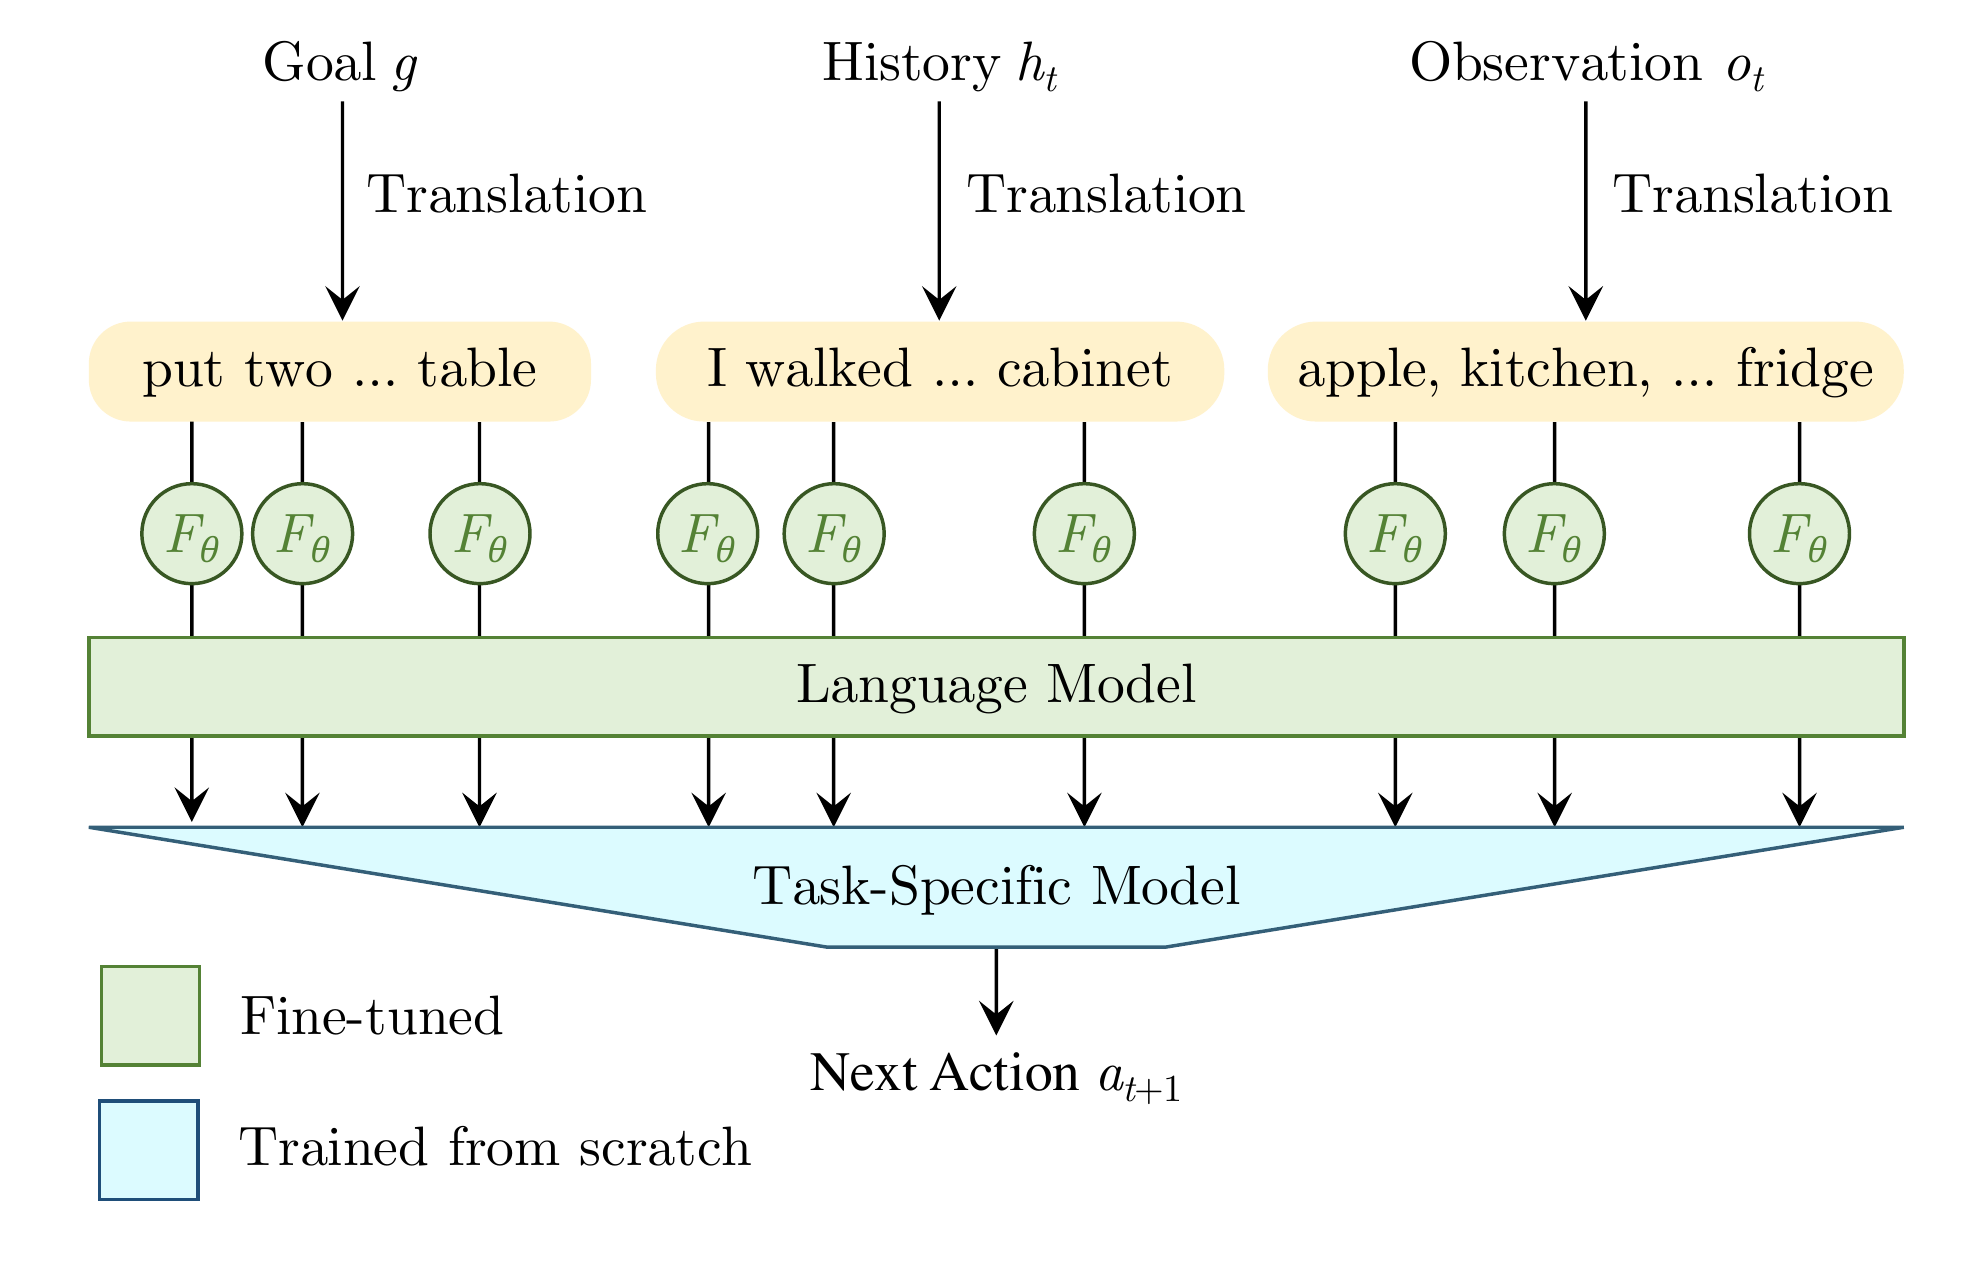}
\end{center}
\vspace{-12pt}
\caption{\small \textbf{Model architecture of the proposed model in the main paper \sect{exp:exp1}}.}
\label{fig:model_repno}
\vspace{-10pt}
\end{figure}
